# Supplementary material for: Radiative decay of an emitter due to non-Markovian interactions with dissipating matter
Source: arXiv:2107.01484 ancillary file (2022-05-23)
Supplement: Supplementary file 1 [file Supplementary_Jain.pdf]

**Supplementary Information:**  
**Radiative decay of an emitter due to non-Markovian interactions**  
**with dissipating matter**

Kritika Jain and Murugesan Venkatapathi\*  
*Computational and Statistical Physics Laboratory,*  
*Indian Institute of Science, Bangalore, 560012*

---

\* muruges@iisc.ac.in

## I. SUMMARY OF ADDITIONAL FIGURES

This supplementary document presents results for different polarizations of the emitter, and other sizes of gold nanoparticles, that add to the more significant results presented in the main paper. Note that Z-axis represents the line joining the center of the metal nano sphere and the point emitter, whereas X and Y are in the plane perpendicular to it. Also, the insensitivity of the results to the strength of the weak coupling of oscillators to vacuum, is highlighted in Figure S12.

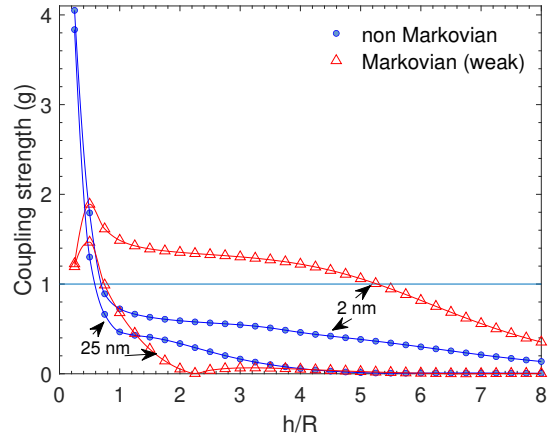

FIG. S1. Coupling strength  $g$  for Z-polarization (initial state of emitter) given by  $\Omega/\Gamma$ , varying with the separation  $h$  of the emitter from the surface of gold particles of radii  $R = 2$  nm and  $R = 25$  nm.

- 
- [1] K. Jain and M. Venkatapathi, “Strong coupling of an emitter with absorbing matter: A regime for enhancement of light emission,” *Phys. Rev. Appl.* **11**, 054002 (2019).

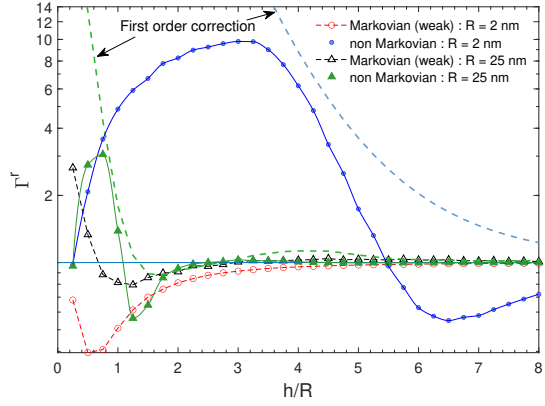

FIG. S2. Radiative decay rates  $\Gamma^r$  for Z-polarization (initial state of emitter) normalized by free-space decay rates  $\Gamma_0^r$  at emission energy  $\hbar\omega_0 = 2.21$  eV when gold nanoparticles are introduced with varying separations  $h$  in a medium of refractive index 1.5. The first order correction of the weak-coupling values for non-Markovian effects on the efficiency [1] is given by the dashed lines. This correction for effective values was given by  $\Gamma_{eff}^r = \Gamma^r + e^{-1/g} \cdot \Gamma_1^{nr}$ , where subscript ‘1’ represents the dipole mode.

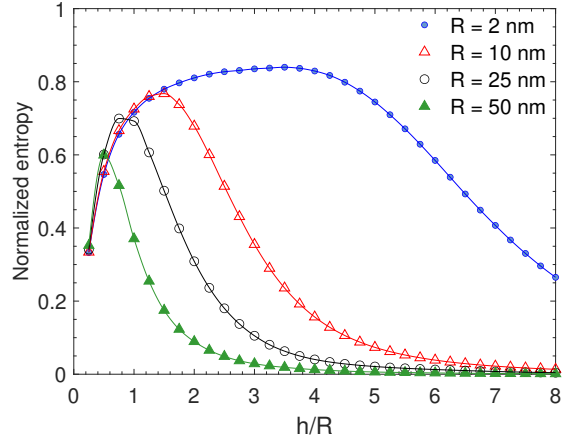

FIG. S3. The normalized von Neumann entropy of the mixture for Z-polarization (initial state of emitter),  $\frac{-1}{\log n} \sum_1^n p_i \log p_i$ , varying with relative separations for particles of different radii  $R$ .  $n$  is 1419 in the evaluations presented.

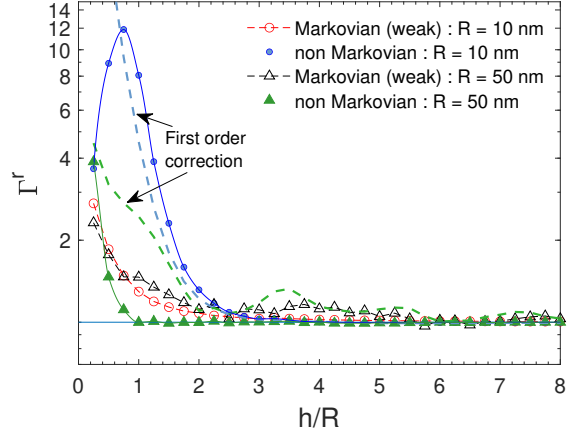

FIG. S4. Radiative decay rates  $\Gamma^r$  for X/Y-polarization (initial state of emitter) normalized by free-space decay rates  $\Gamma_0^r$  at emission energy  $\hbar\omega_0 = 2.21$  eV when gold nanoparticles are introduced with varying separations  $h$  in a medium of refractive index 1.5. The first order correction of the weak-coupling values for non-Markovian effects on the efficiency [1] is given by the dashed lines. This correction for effective values was given by  $\Gamma_{eff.}^r = \Gamma^r + e^{-1/g} \cdot \Gamma_1^{nr}$ , where subscript ‘1’ represents the dipole mode.

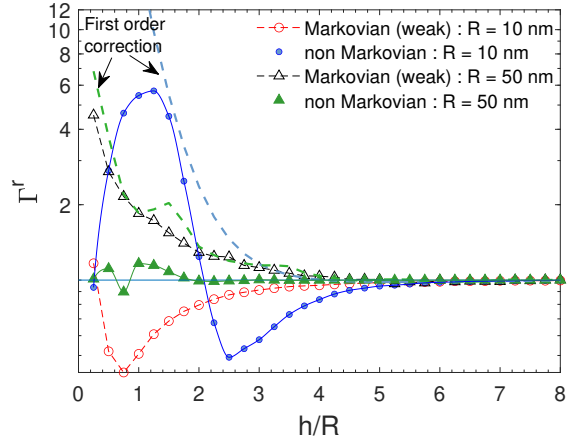

FIG. S5. Radiative decay rates  $\Gamma^r$  for Z-polarization (initial state of emitter) normalized by free-space decay rates  $\Gamma_0^r$  at emission energy  $\hbar\omega_0 = 2.21$  eV when gold nanoparticles are introduced with varying separations  $h$  in a medium of refractive index 1.5. The first order correction of the weak-coupling values for non-Markovian effects on the efficiency [1] is given by the dashed lines. This correction for effective values was given by  $\Gamma_{eff.}^r = \Gamma^r + e^{-1/g} \cdot \Gamma_1^{nr}$ , where subscript ‘1’ represents the dipole mode.

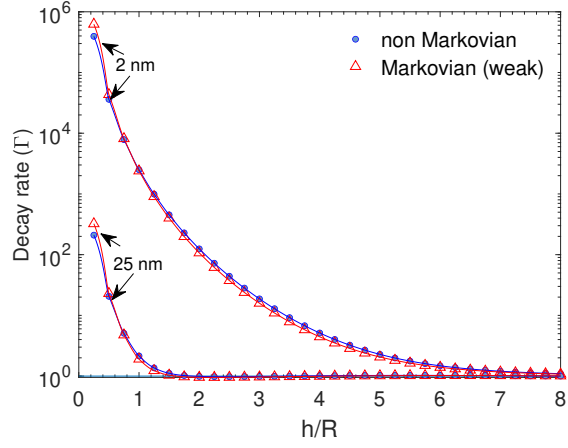

FIG. S6. Total decay rates  $\Gamma$  for X/Y-polarization (initial state of emitter) normalized by free-space decay rates  $\Gamma_0^r$  at emission energy  $\hbar\omega_0 = 2.21$  eV when gold nanoparticles of radii 2 nm and 25 nm are introduced with varying separations  $h$  in a medium of refractive index 1.5.

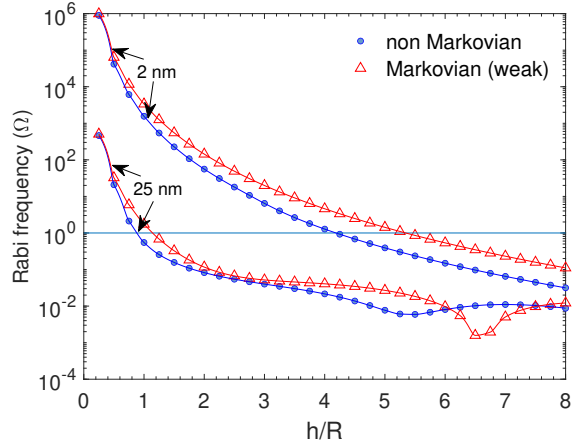

FIG. S7. Rabi frequency  $\Omega$  for X/Y-polarization (initial state of emitter) normalized by free-space decay rates  $\Gamma_0^r$  at emission energy  $\hbar\omega_0 = 2.21$  eV when gold nanoparticles of radii 2 nm and 25 nm are introduced with varying separations  $h$  in a medium of refractive index 1.5.

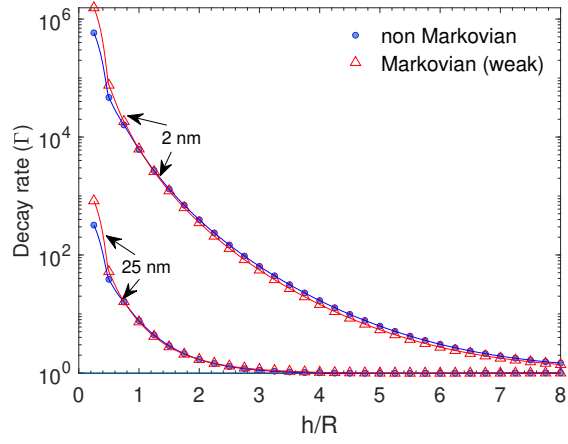

FIG. S8. Total decay rates  $\Gamma$  for Z-polarization (initial state of emitter) normalized by free-space decay rates  $\Gamma_0^r$  at emission energy  $\hbar\omega_0 = 2.21$  eV when gold nanoparticles of radii 2 nm and 25 nm are introduced with varying separations  $h$  in a medium of refractive index 1.5.

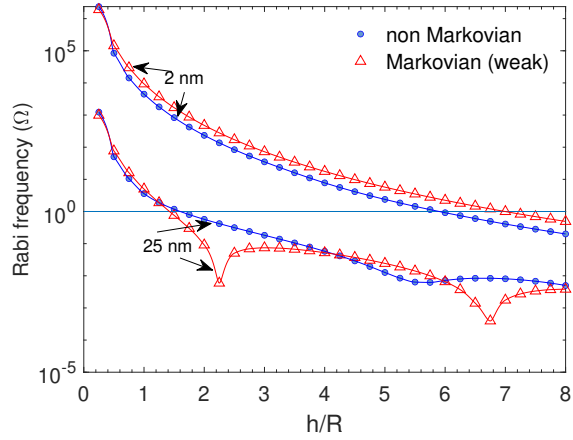

FIG. S9. Rabi frequency  $\Omega$  for Z-polarization (initial state of emitter) normalized by free-space decay rates  $\Gamma_0^r$  at emission energy  $\hbar\omega_0 = 2.21$  eV when gold nanoparticles of radii 2 nm and 25 nm are introduced with varying separations  $h$  in a medium of refractive index 1.5.

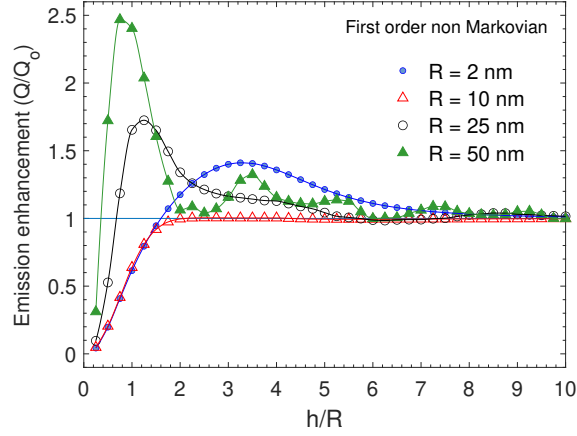

FIG. S10. Normalized quantum efficiencies for X/Y-polarization (initial state of emitter) show enhancement of  $Q$  for the smallest and large gold nanoparticle and no enhancement for 10 nm particle, in the case of the first order corrections to the Markovian model for the non-Markovian effects.  $Q_0=1/3$  was assumed, and the enhancements have an inverse relationship with  $Q_0$ . The first order correction for effective values was given by  $\Gamma_{eff}^r = \Gamma^r + e^{-1/g} \cdot \Gamma_1^{nr}$  and  $\Gamma_{eff}^{nr} = \Gamma^{nr} - e^{-1/g} \cdot \Gamma_1^{nr}$ , where subscript ‘1’ represents the dipole mode.

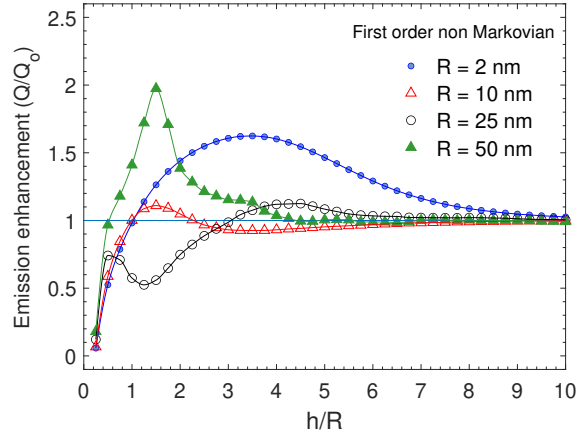

FIG. S11. Normalized quantum efficiencies for Z-polarization (initial state of emitter) show more enhancement of  $Q$  for the smallest and largest gold nanoparticle, in the case of the first order corrections to the Markovian model for the non-Markovian effects.  $Q_0=1/3$  was assumed, and the enhancements have an inverse relationship with  $Q_0$ . The first order correction for effective values was given by  $\Gamma_{eff}^r = \Gamma^r + e^{-1/g} \cdot \Gamma_1^{nr}$  and  $\Gamma_{eff}^{nr} = \Gamma^{nr} - e^{-1/g} \cdot \Gamma_1^{nr}$ , where subscript ‘1’ represents the dipole mode.

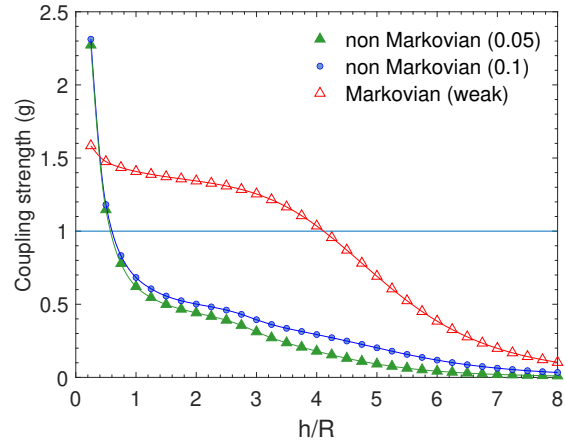

FIG. S12. Change in the coupling strength  $g$  of emitter with the gold particle of 2nm radius, due to a variation of the coupling strength of the isolated oscillators and vacuum
